# Supplementary material for: Realization of distance matrices by graphs of genus 1
Source: arXiv:2012.07698 ancillary file (2020-12-14)
Supplement: Supplementary file 1 [file Description_of_procedures_in_Maple.pdf]

# Description of the procedures in Maple

## 1 Subprocedures for compaction vector and matrix

### 1.1 CV

The procedure **CV** takes in input a distance matrix  $M$  and produces, in output, its compaction vector. It is invoked by the command **CV(M)**.

### 1.2 CM

The procedure **CM** takes, in input, a distance matrix  $M$  and its compaction vector  $V$  and produces, in output, the compaction matrix of  $M$  with respect to  $V$ . It is invoked by the command **CM(M,V)**.

## 2 RedMat

The procedure **RedMat** takes in inputs a matrix  $M$  and analyses its equal rows and columns. The output is a matrix of size  $(2t + 1) \times d$  where

- $t$  is the maximal cardinality of a set of indices of equal rows and columns,
- $d$  is the total number of distinct sets of indices of equal rows and columns,
- the  $(t + 1)$ -th column contains the cardinality of each set of indices of equal rows and columns,
- the rightmost  $d \times t$  matrix contains, in each row, the indices of equal rows and columns.

It is invoked by the command **RedMat(M)**.

### 3 Procedures to check realization by an $n$ -cycle

#### 3.1 AP

The procedure **AP** takes in input a distance matrix  $M$  of size  $n \times n$  and checks, over all permutations of  $n$  elements, if there is one permutation that satisfies the formulas for  $M$  being realizable by an  $n$ -cycle. If so, **AP** returns that permutation. If not, it returns an empty list. This is a procedure with high computational cost as  $n$  grows. It is invoked by the command **AP(M)**.

#### 3.2 EP

The procedure **EP** takes in input a distance matrix  $M$  of size  $n \times n$  and tries to find an expected permutation that satisfies the formulas for  $M$  being realizable by an  $n$ -cycle. If so, **EP** returns that permutation. If not it returns an empty list. It is invoked by the command **EP(M)**.

### 4 The main procedure

The procedure **G1RG** takes in input a distance matrix  $M$  and analyses if it is realizable by a tree or a graph of genus 1. If so, it returns a graph which can be seen using the command **DrawGraph(G, style = spring)**, where  $G$  is assigned invoking the procedure by the command **G:=G1RG(M)**.

**G1RG** accepts two optional arguments **OutData** and **FindPerm**, in the form **G1RG(M, OutData, FindPerm)**. If **OutData=1** (default 0), **G1RG** prints, for each step of the algorithm, the compaction vector, the equal rows and columns in the compaction matrix and the weighted adjacency matrix of the resulting graph. In the case of a realization by a graph of genus 1, prints the order of the nodes in the internal cycle. If **FindPerm=1** (default 0), **G1RG** uses the subprocedure **AP**, instead of **EP**.
